# Supplementary material for: Strong coupling of lattice and orbital excitations in quantum magnet Ca$_{10}$Cr$_7$O$_{28}$: Anomalous temperature dependence of Raman phonons
Source: arXiv:2308.03237 ancillary file (2023-08-07)
Supplement: Supplementary file 1 [file SI.pdf]

**Supplementary Material: Strong coupling of lattice and orbital  
excitations in quantum magnet  $\text{Ca}_{10}\text{Cr}_7\text{O}_{28}$ : Anomalous  
temperature dependence of Raman phonons**

Srishti Pal,<sup>1,\*</sup> Arnab Seth,<sup>2,3</sup> Anzar Ali,<sup>4</sup> Yogesh Singh,<sup>4</sup>

D. V. S. Muthu,<sup>1</sup> Subhro Bhattacharjee,<sup>2</sup> and A. K. Sood<sup>1</sup>

<sup>1</sup>*Department of Physics, Indian Institute of Science, Bengaluru 560012, India*

<sup>2</sup>*International Centre for Theoretical Sciences,*

*Tata Institute of Fundamental Research, Bengaluru 560089, India*

<sup>3</sup>*School of Physics, Georgia Institute of Technology, Atlanta, GA 30332, USA*

<sup>4</sup>*Indian Institute of Science Education and Research (IISER) Mohali,*

*Knowledge City, Sector 81, Mohali 140306, India*

## S1. SAMPLE AND EXPERIMENTAL METHODS

Polycrystalline samples of  $\text{Ca}_{10}\text{Cr}_7\text{O}_{28}$  were synthesized from  $\text{CaCO}_3$  and  $\text{Cr}_2\text{O}_3$  powders (99.99%, Alfa-Aesar) by a conventional solid state reaction method as described in detail previously.<sup>1</sup> As reported earlier,  $\text{Ca}_{10}\text{Cr}_7\text{O}_{28}$  consists of two kagome planes of the breathing bilayer consists of two inequivalent corner-sharing triangles with alternating ferromagnetic (FM) and antiferromagnetic (AFM) couplings in the *ab*-plane. The FM triangles of one kagome plane lie directly above the AFM triangles of the next one and these bi-triangles are then ferromagnetically coupled to form the bilayer kagome structure giving rise to moderate frustration in this complex spin-system.<sup>2,3</sup>

Unpolarized Raman spectra on the polycrystalline samples of  $\text{Ca}_{10}\text{Cr}_7\text{O}_{28}$  were recorded using laser of wavelength 691 nm. The spectra were collected in a backscattering geometry using Horriba LabRAM HR Evolution Spectrometer equipped with a thermoelectric cooled charge coupled device (CCD) (HORIBA Jobin Yvon, SYNCERITY  $1024 \times 256$ ). The low temperature Raman measurements from 4 K to 295 K were performed with closed cycle He cryostat (Cryostation S50, Montana Instruments) with a temperature stability of  $\approx \pm 1$  K.

## S2. LATTICE ANHARMONICITY

The orange curves in Figure 2 of the main text are fits to cubic anharmonic model given by,

$$\omega_{anh}^{(p)} = \omega_0 + A \left[ 1 + 2n \left( \frac{\omega_0}{2} \right) \right] \quad (\text{S1})$$

$$\Pi_{anh}^{(p)} = \Gamma_0 + B \left[ 1 + 2n \left( \frac{\omega_0}{2} \right) \right] \quad (\text{S2})$$

where,  $\omega_0$  and  $\Gamma_0$  are frequencies and linewidths at absolute zero,  $A$  (negative) and  $B$  (positive) are constants, and  $n \left( \frac{\omega_0}{2} \right)$  is the Bose-Einstein thermal factor. The  $\omega_0$  values for different modes have been extracted from the frequency fits in the temperature range of 110 - 295 K and then those values are used to fit the FWHMs. The values for the fitting parameters  $\omega_0$ ,  $\Gamma_0$ ,  $A$ , and  $B$  for selected modes are shown in Table S1.

**Table S1:** List of parameters for the cubic anharmonic fits to the phonon modes of  $\text{Ca}_{10}\text{Cr}_7\text{O}_{28}$ 

| Mode | $\omega_0$ ( $\text{cm}^{-1}$ ) | $A$    | $\Gamma_0$ ( $\text{cm}^{-1}$ ) | $B$  |
|------|---------------------------------|--------|---------------------------------|------|
| M1   | 326.8                           | - 2.4  | 38.4                            | 4.7  |
| M2   | 363.2                           | - 1.7  | 13.0                            | 6.3  |
| M5   | —                               | —      | 34.4                            | 7.3  |
| M6   | —                               | —      | 5.1                             | 17.7 |
| M8   | 888                             | - 15.9 | 9.1                             | 23.9 |

### S3. INTEGRATED SUSCEPTIBILITIES OF PHONON MODES

The susceptibility  $\chi(\omega)$  for the phonon modes have been extracted from their integrated intensities  $I(\omega)$  using the relation,  $I(\omega) \propto [1 + n(\omega)]\chi(\omega)$  where,  $1 + n(\omega) = 1/[1 - e^{-\hbar\omega/k_B T}]$  is the Bose-Einstein thermal population factor. The temperature evolution of the integrated susceptibilities for selected phonon modes are shown in Fig. S1. The sharp increase in the susceptibilities for modes M1, M5, and M6 with decreasing temperatures is indicative of enhanced dipole Raman matrix element as seen in cuprate superconductors.<sup>4</sup>

### S4. JAHN-TELLER DISTORTED TETRAHEDRA

Figure S2 shows the distorted  $\text{Cr}^V\text{O}_4$  tetrahedra of  $\text{Ca}_{10}\text{Cr}_7\text{O}_{28}$  at two crystallographically inequivalent sites Cr1 and Cr2.<sup>5</sup>

### S5. THE SECONDARY J-T TRANSITION AND ORBITAL RE-ORDERING

On lowering the temperature from the primary JT temperature scale, as discussed in the main text, the secondary JT couplings tries to modify the splitting scheme as favoured by  $K_{ij}^{\alpha\beta}$ . This leads to reorientation of the orbital ordering from  $\langle\tau^z\rangle \neq 0$ . The qualitative effects on the orbital can be easily captured by the CW mean field theory.<sup>6</sup> Assuming the simplified case where the cooperative JT tries to align the orbitals, we can determine the

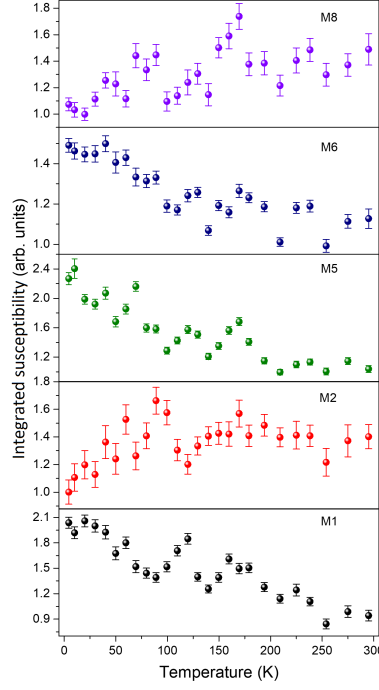

**Figure S1:** Temperature variation of the integrated susceptibilities of selected phonon modes.

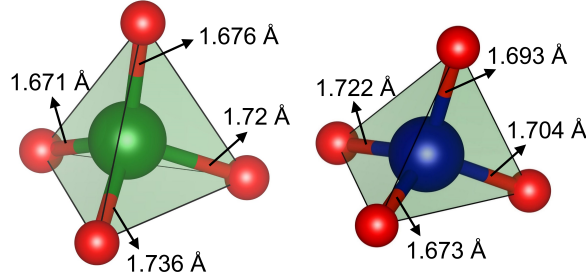

**Figure S2:** J-T distorted  $\text{Cr}^{\text{V}}\text{O}_4$  tetrahedra of  $\text{Ca}_{10}\text{Cr}_7\text{O}_{28}$  at two  $\text{Cr}^{5+}$  sites Cr1 (Green) and Cr2 (Blue).

mean field phase diagram, which is shown in Figure S3.

## S6. COUPLING BETWEEN ORBITAL AND LATTICE DEGREES OF FREEDOM

The coupling constant,  $\mathcal{K}^{\alpha\beta}$ , are dependent on the dynamic distortions of the tetrahedra in the JT distorted state as given in Eq. 3 of the main text. Putting this back in the purely orbital part of the Hamiltonian given in Eq. 2 of the main text, we get the coupling between

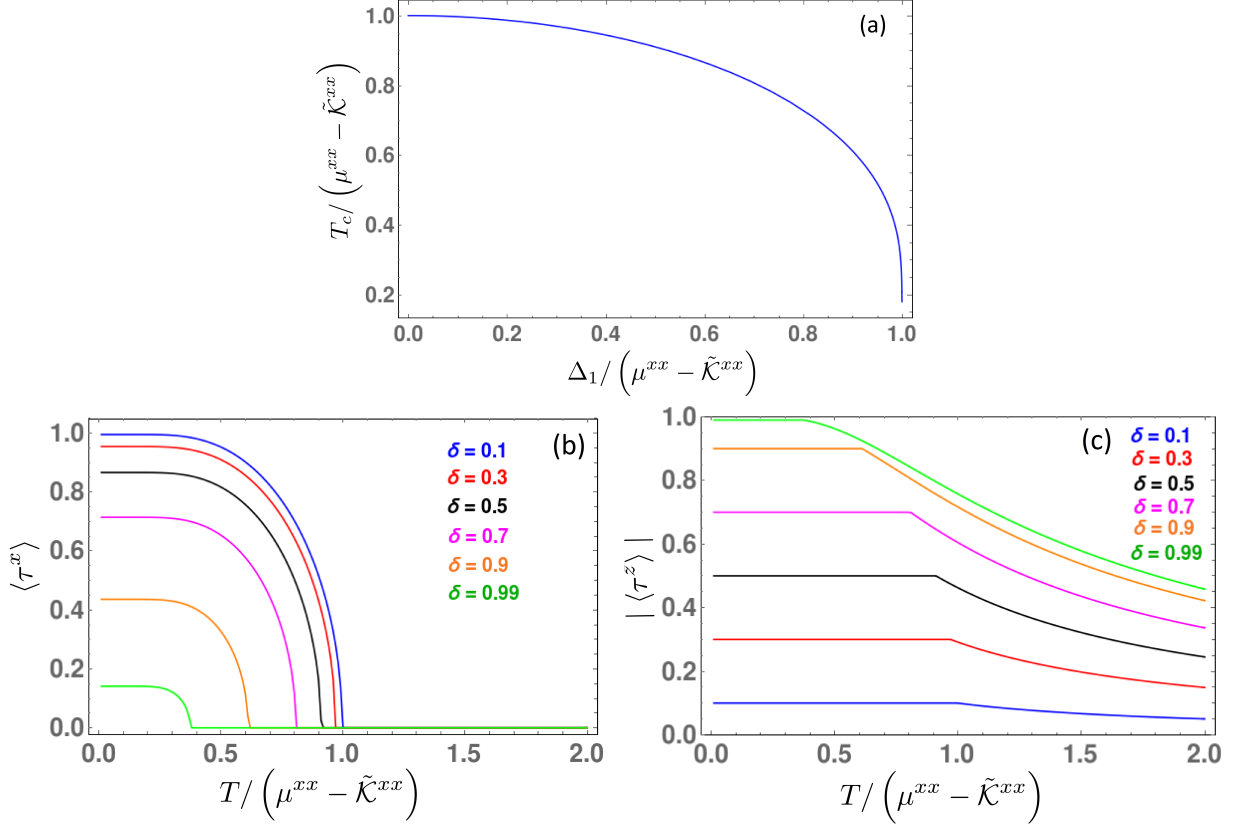

**Figure S3:** Orbital reordering due to the cooperative Jahn-Teller transition. (a) Temperature scale associated with the orbital reordering transition. (b)  $\tau^x$  vs temperature. (c)  $|\tau^z|$  vs temperature.

phonon and orbital degrees of freedom.

$$\bar{H} = H_{orb} + H_{orb-ph} \quad (S3)$$

where,

$$H_{orb} = \sum_{ij} \bar{\kappa}_{ij}^{\alpha\beta} \tau_i^\alpha \tau_j^\beta + \Delta_1 \sum_i \tau_i^z \quad (S4)$$

$$H_{orb-ph} = \sum_i \left[ \Gamma^{p,\beta} \tau_i^\beta + \sum_j A_{ij}^{\alpha\beta;p} \tau_i^\alpha \tau_j^\beta \right] \epsilon_i^p + \sum_{ij} B_{ij}^{\alpha\beta;pq} \tau_i^\alpha \tau_j^\beta \epsilon_i^p \epsilon_j^q \quad (S5)$$

where,  $A_{ij}^{\alpha\beta;p}$  and  $B_{ij}^{\alpha\beta;pq}$  are given by Eq. 3 in the main text.

## S7. THE PHONON LINEWIDTH

$$\begin{aligned}
\Pi_{orb}^{(p)} \propto \text{Im} \left( \int_0^\beta d\tau e^{i\omega_n \tau} \left[ \Gamma^{(p)\beta} \Gamma^{(p)\beta'} \sum_{ij} \langle \langle \hat{T} \left( \tau_i^\beta(\tau) \tau_j^{\beta'}(0) \right) \rangle \rangle + \Gamma^{(p)\beta} \sum_{ijk} A_{jk}^{\beta'\gamma';(p)} \langle \langle \hat{T} \left( \tau_i^\beta(t) \tau_j^{\beta'}(0) \tau_k^{\gamma'}(0) \right) \rangle \rangle \right. \right. \\
+ \sum_{ijk} A_{ij}^{\beta\gamma;(p)} \Gamma^{(p)\beta'} \langle \langle \hat{T} \left( \tau_i^\beta(\tau) \tau_j^\gamma(\tau) \tau_k^{\beta'}(0) \right) \rangle \rangle \\
\left. \left. + \sum_{ijkl} A_{ij}^{\beta\gamma;(p)} A_{kl}^{\beta'\gamma';(p)} \langle \langle \hat{T} \left( \tau_i^\beta(\tau) \tau_j^\gamma(\tau) \tau_k^{\beta'}(0) \tau_l^{\gamma'}(0) \right) \rangle \rangle \right] \right)_{i\omega_n \rightarrow \omega + i0^+} \quad (S6)
\end{aligned}$$

There are three contributions proportional to  $\mathcal{O}(\Gamma^2)$ ,  $\mathcal{O}(\Gamma A)$  and  $\mathcal{O}(A^2)$  which are rearranged to obtain :

$$\begin{aligned}
\Pi_{orb}^{(p)}(\mathbf{k} = 0, \omega) = \sum_{\mu, \nu=x,z} \mathcal{M}_{\mu\nu} \text{Im} \left[ \tilde{\mathcal{C}}_{\mu\nu}(\mathbf{k} = 0, \omega + i0^+) \right] \\
+ \sum_{\mu, \nu=x,z} \sum_{\alpha, \beta=x,z} \mathcal{M}_{\alpha\beta\mu\nu} \text{Im} \left[ \int d\mathbf{k}' \sum_m \tilde{\mathcal{C}}_{\mu\nu}(\mathbf{k}', \Omega_m + \omega_n) \tilde{\mathcal{C}}_{\alpha\beta}(-\mathbf{k}', -\Omega_m) \right] \quad (S7)
\end{aligned}$$

$$\begin{aligned}
\mathcal{M}_{\mu\nu} = \Gamma^{p,\mu} \Gamma^{p,\nu} + \Gamma^{p,\mu} (A^{\nu\alpha;p} + A^{\alpha\nu;p}) \langle \tau^\alpha \rangle \\
+ \Gamma^{p,\nu} (A^{\mu\alpha;p} + A^{\alpha\mu;p}) \langle \tau^\alpha \rangle + (A^{\mu\alpha;p} A^{\nu\beta;p} + A^{\mu\alpha;p} A^{\beta\nu;p}) \langle \tau^\alpha \rangle \langle \tau^\beta \rangle \quad (S8)
\end{aligned}$$

$$\mathcal{M}_{\alpha\beta\mu\nu} = \frac{1}{2\pi} (A^{\mu\alpha;p} A^{\nu\beta;p} + A^{\mu\alpha;p} A^{\beta\nu;p}) \quad (S9)$$

Here  $M_{\mu\nu}$  and  $M_{\alpha\beta\mu\nu}$  are in general temperature dependent coupling coefficients. It is clear from the above expression that the various contributions, within the the quadratic approximations are given by the various components of the two-spin correlation function  $\tilde{\mathcal{C}}_{\mu\nu}(\mathbf{k}, i\omega_n)$  which we now calculate within quadratic approximation using the low energy orbital hamiltonian  $H_{orb}$  (Eq. S4).

## S8. TIME-ORDERED CORRELATION FUNCTIONS FOR THE ORBITAL DEGREES OF FREEDOM IN IMAGINARY TIME FORMULATION

Equations of motion for the correlators can be obtained from those of the spins and are given by :

$$\dot{\mathcal{C}}_{xx}(\mathbf{r}, t) = 2i\Delta_1 \mathcal{C}_{yx}(\mathbf{r}, t) \quad (\text{S10})$$

$$\dot{\mathcal{C}}_{yx}(\mathbf{r}, t) + 2i\Delta_1 \mathcal{C}_{xx}(\mathbf{r}, t) = -2i\delta(t)\delta(\mathbf{r})\langle\tau^z\rangle - 2i\Delta_1\langle\tau^x\rangle^2 + 2i\bar{\mathcal{K}}^{xx} \sum_{\mathbf{d}} \langle \hat{T}(\tau_{\mathbf{r}}^z(t)\tau_{\mathbf{r}+\mathbf{d}}^x(t)\tau_0^x(0)) \rangle \quad (\text{S11})$$

$$\dot{\mathcal{C}}_{zx}(\mathbf{r}, t) = -2i\bar{\mathcal{K}}^{xx} \sum_{\mathbf{d}} \langle \hat{T}(\tau_{\mathbf{r}}^y(t)\tau_{\mathbf{r}+\mathbf{d}}^x(t)\tau_0^x(0)) \rangle \quad (\text{S12})$$

$$\dot{\mathcal{C}}_{yz}(\mathbf{r}, t) = 2i\delta(t)\delta(\mathbf{r})\langle\tau^x\rangle + 2i\bar{\mathcal{K}}^{xx} \sum_{\mathbf{d}} \langle \hat{T}(\tau_{\mathbf{r}}^z(t)\tau_{\mathbf{r}+\mathbf{d}}^x(t)\tau_0^z(0)) \rangle - 2i\Delta_1 (\mathcal{C}_{xz}(\mathbf{r}, t) + \langle\tau^x\rangle\langle\tau^z\rangle) \quad (\text{S13})$$

$$\dot{\mathcal{C}}_{zz}(\mathbf{r}, t) = -2i\bar{\mathcal{K}}^{xx} \sum_{\mathbf{d}} \langle \hat{T}(\tau_{\mathbf{r}}^y(t)\tau_{\mathbf{r}+\mathbf{d}}^x(t)\tau_0^z(0)) \rangle \quad (\text{S14})$$

$$\dot{\mathcal{C}}_{xz}(\mathbf{r}, t) = 2i\Delta_1 \mathcal{C}_{yz}(\mathbf{r}, t) \quad (\text{S15})$$

## Quadratic Approximations and solving the equations of motion of time-ordered correlation function

**Approximation 1:** To solve the above equations of motion, we approximate the 3-point correlators in the above equations of motion by splitting into 2-point and 1-point correlations. A typical example looks like as follows.

$$\bar{\mathcal{K}}^{xx} \sum_{\mathbf{d}} \langle \hat{T}(\tau_{\mathbf{r}}^z(t)\tau_{\mathbf{r}+\mathbf{d}}^x(t)\tau_0^x(0)) \rangle \approx \tilde{\mathcal{K}}^{xx} (\langle \langle \tau_{\mathbf{r}}^z \tau_{\mathbf{r}+\mathbf{d}}^x \rangle \rangle \langle \tau^x \rangle + \mathcal{C}_{zx}(\mathbf{r}, t) \langle \tau^x \rangle + \mathcal{C}_{xx}(\mathbf{r}, t) \langle \tau^z \rangle + \langle \tau^z \rangle \langle \tau^x \rangle^2) \quad (\text{S16})$$

where,  $\tilde{\mathcal{K}}^{xx} = \bar{\mathcal{K}}^{xx} D$  with  $D$  being the coordination number. The first term is time-independent, hence do not contribute to finite frequency response.

**Approximation 2:** We further do a second approximation by setting the nearest neighbour 2-point correlator in Eq. S16 to its mean field value, such that,  $\langle \langle \tau_{\mathbf{r}}^z \tau_{\mathbf{r}+\mathbf{d}}^x \rangle \rangle = \langle \tau_{\mathbf{r}}^z \tau_{\mathbf{r}+\mathbf{d}}^x \rangle - \langle \tau_{\mathbf{r}}^z \rangle \langle \tau_{\mathbf{r}+\mathbf{d}}^x \rangle \approx 0$ .

With these approximations, the equation of motions can be remarkably simplified. Further going into the frequency domain, the differential equations turn into algebraic equations, which are straightforward to solve. The correlation function in frequency domain is given by,

$$\tilde{C}_{yz}(i\omega_n, \mathbf{k} = 0) = -\frac{i\omega_n \tilde{C}_1(i\omega_n, \mathbf{k} = 0)}{(i\omega_n)^2 - \left(4\Delta_1^2 + 4\tilde{\mathcal{K}}^{xx^2}\langle\tau^x\rangle^2 - 4\tilde{\mathcal{K}}^{xx}\Delta_1\langle\tau^z\rangle\right) - \Gamma^2 - 2\omega_n\Gamma} \quad (\text{S17})$$

$$\tilde{C}_{xz}(i\omega_n, \mathbf{k} = 0) = \frac{2i\Delta_1 \tilde{C}_1(i\omega_n, \mathbf{k} = 0)}{(i\omega_n)^2 - \left(4\Delta_1^2 + 4\tilde{\mathcal{K}}^{xx^2}\langle\tau^x\rangle^2 - 4\tilde{\mathcal{K}}^{xx}\Delta_1\langle\tau^z\rangle\right) - \Gamma^2 - 2\omega_n\Gamma} \quad (\text{S18})$$

$$\tilde{C}_{zz}(i\omega_n, \mathbf{k} = 0) = -\frac{2i\tilde{\mathcal{K}}^{xx}\langle\tau^x\rangle \tilde{C}_1(i\omega_n, \mathbf{k} = 0)}{(i\omega_n)^2 - \left(4\Delta_1^2 + 4\tilde{\mathcal{K}}^{xx^2}\langle\tau^x\rangle^2 - 4\tilde{\mathcal{K}}^{xx}\Delta_1\langle\tau^z\rangle\right) - \Gamma^2 - 2\omega_n\Gamma} \quad (\text{S19})$$

$$\tilde{C}_{yx}(i\omega_n, \mathbf{k} = 0) = -\frac{i\omega_n \tilde{C}_2(i\omega_n, \mathbf{k} = 0)}{(i\omega_n)^2 - \left(4\Delta_1^2 + 4\tilde{\mathcal{K}}^{xx^2}\langle\tau^x\rangle^2 - 4\tilde{\mathcal{K}}^{xx}\Delta_1\langle\tau^z\rangle\right) - \Gamma^2 - 2\omega_n\Gamma} \quad (\text{S20})$$

$$\tilde{C}_{xx}(i\omega_n, \mathbf{k} = 0) = \frac{2i\Delta_1 \tilde{C}_2(i\omega_n, \mathbf{k} = 0)}{(i\omega_n)^2 - \left(4\Delta_1^2 + 4\tilde{\mathcal{K}}^{xx^2}\langle\tau^x\rangle^2 - 4\tilde{\mathcal{K}}^{xx}\Delta_1\langle\tau^z\rangle\right) - \Gamma^2 - 2\omega_n\Gamma} \quad (\text{S21})$$

$$\tilde{C}_{zx}(i\omega_n, \mathbf{k} = 0) = -\frac{2i\tilde{\mathcal{K}}^{xx}\langle\tau^x\rangle \tilde{C}_2(i\omega_n, \mathbf{k} = 0)}{(i\omega_n)^2 - \left(4\Delta_1^2 + 4\tilde{\mathcal{K}}^{xx^2}\langle\tau^x\rangle^2 - 4\tilde{\mathcal{K}}^{xx}\Delta_1\langle\tau^z\rangle\right) - \Gamma^2 - 2\omega_n\Gamma} \quad (\text{S22})$$

where,

$$\tilde{C}_1(i\omega_n, \mathbf{k} = 0) = \frac{2i}{N}\langle\tau^x\rangle + 2i\beta\langle\tau^x\rangle\langle\tau^z\rangle \left(\tilde{\mathcal{K}}^{xx}\langle\tau^z\rangle - \Delta_1\right) \delta_{n,0}$$

$$\tilde{C}_2(i\omega_n, \mathbf{k} = 0) = -\frac{2i}{N}\langle\tau^z\rangle + 2i\beta\langle\tau^x\rangle^2 \left(\tilde{\mathcal{K}}^{xx}\langle\tau^z\rangle - \Delta_1\right) \delta_{n,0}$$

and we have added a phenomenological damping,  $\Gamma$  which causes the temporal decay of correlation functions.

The correlators in the real frequency space can be obtained from the above by the standard procedure of analytic continuation,  $i\omega_n \rightarrow \omega + i0^+$ .

The imaginary part of the above correlation functions contribute to the phonon linewidth as described in Eq. 7 of the main text. Since the numerators of the above expressions are purely real, the contribution completely comes from the denominator. Generically, all the contribution looks like as follows,

$$\text{Im} \left[ \tilde{C}_{\mu\nu}(\omega + i0^+, \mathbf{k} = 0) \right] \propto -\frac{2\omega\Gamma}{\left(\omega^2 - \left(4\Delta_1^2 + 4\tilde{\mathcal{K}}^{xx^2}\langle\tau^x\rangle^2 - 4\tilde{\mathcal{K}}^{xx}\Delta_1\langle\tau^z\rangle\right) - \Gamma^2\right)^2 + 4\omega^2\Gamma^2} \quad (\text{S23})$$

Substituting the above in Eq. S7, we obtain the renormalisation of the linewidth of the phonons.

---

\* E-mail: [srishtipal@iisc.ac.in](mailto:srishtipal@iisc.ac.in)

- <sup>1</sup> A. Balodhi and Y. Singh, *Phys. Rev. Mater.* **1**, 024407 (2017).
- <sup>2</sup> C. Balz, B. Lake, A. T. M. N. Islam, Y. Singh, J. A. Rodriguez-Rivera, T. Guidi, E. M. Wheeler, G. G. Simeoni, and H. Ryll, *Phys. Rev. B* **95**, 174414 (2017).
- <sup>3</sup> C. Balz, B. Lake, M. Reehuis, A. T. M. N. Islam, O. Prokhnenko, Y. Singh, P. Pattison, and S. Tóth, *J. Phys.: Condens. Matter* **29**, 225802 (2017).
- <sup>4</sup> O. V. Misochko, E. Y. Sherman, N. Umesaki, K. Sakai, and S. Nakashima, *Phys. Rev. B* **59**, 11495 (1999).
- <sup>5</sup> D. Gyepesová and V. Langer, *Acta Cryst.* **C69**, 111 (2013).
- <sup>6</sup> R. B. Stinchcombe, *Journal of Physics C: Solid State Physics* **6**, 2459 (1973).
